# Supplementary material for: Discrete Beamforming Optimization for RISs with a Limited Phase Range and Amplitude Attenuation
Source: arXiv:2507.07342 source file (2025-07-09)
Supplement: Supplementary file 1 [file appendixb.tex]

\section{Element-Based Simple Update Rule}
We now further simplify Algorithm~2, so that there is no need for calculating $s_{nk}$ or $\lambda_l .$
What we need to have is, given an initial $\phase{\mu}$ selection, say $e^{j \small \phase{\mu}\normalsize} \in {\rm arc}
(e^{j\lambda_{i-1}}:e^{j\lambda_i}),$ we want to know the $N$-step update rule ${\cal N}(\lambda_l),
l=i,i+1,\ldots,i+N-1$ in the for loop of Algorithm~2.

{\em Claim:\/} Let ${\cal U}$ be the set to define the $N$ consecutive updates in the for loop of Algorithm~2.
For an initial $\phase{\mu_0}$ selection, the update rule in the for loop of Algorithm~2 will be ${\cal U} = \{ n_1,n_2,
\ldots, n_N | 0\le \varphi_{n_1} < \varphi_{n_2} < \cdots < \varphi_{n_N} < \frac{2\pi}{K}, \varphi_n =
(\alpha_n - \phase{\mu_0} + \frac{\pi}{K}) \;{\rm mod}\; \frac{2\pi}{K}, n = 1,2, \ldots, N\}$.

{\em Proof:\/}
\begin{comment}
Due to space limitations, we will omit the proof from this version of the paper. We will add it to the
final version in the conference proceedings.
\end{comment}
First, consider the case when $\phase{\mu} = 0.$ We know that the initial arc is
${\rm arc}(e^{j\lambda_L}:e^{j\lambda_1})$. Therefore, the update rule must be
${\cal U} = ({\cal N}(\lambda_l))_{l=1}^N$. We have already calculated this in (\ref{eqn:eqn387}) for any
Case $i$ given in (\ref{eqn:eqn34}). Note, from (\ref{eqn:eqn34}) to (\ref{eqn:eqn387}),
$({\cal N}(\lambda_l))_{l=1}^{NK}$ follows from the indexes of the
sorted values of
\begin{equation}
\varphi_n = \left(\alpha_n+\frac{\pi}{K}\right) \;{\rm mod}\; \frac{2\pi}{K} .
\label{eqn:appb1}
\end{equation}
Now, consider the case when $\phase{\mu} = \phase{\mu_0}$ where $e^{j \small \phase{\mu_0} \normalsize} \notin {\rm arc}(e^{j\lambda_L}:e^{j\lambda_1})$. In this case,
instead of moving $\mu$ to a new arc, we can introduce an offset of $-\phase{\mu_0}$ for all $\lambda_l$.
Note that this corresponds to $\alpha_n\rightarrow \alpha_n - \phase{\mu_0},$ for all $n$. Therefore
(\ref{eqn:appb1}) will be updated as
\begin{equation}
\varphi_n = \left(\alpha_n - \phase{\mu_0} + \frac{\pi}{K}\right)\; {\rm mod}\; \frac{2\pi}{K}.
\label{eqn:appb2}
\end{equation}
Thus, the proof is complete.$\hfill\blacksquare$

Now, when $h_0 \neq 0$, to initialize with $\phase{\mu} = \alpha_0 - \frac{\pi}{K}$, we can simply insert $\phase{\mu_0}
= \alpha_0 -\frac{\pi}{K}$ in (\ref{eqn:appb2}) and get
\begin{equation}
\varphi_n = (\alpha_n - \alpha_0) \;{\rm mod}\; \frac{2\pi}{K}\label{eqn:eqn42}
\end{equation}
to be used in the initialization step. When the BS-UE link
is completely blocked, or $h_0=0$, initializations can be updated as $\phase{\mu}=0$ in Step~4 and
$\varphi_n = \left(\alpha_n-\frac{\pi}{K}\right)\; {\rm mod}\; \frac{2\pi}{K}$ for $n=1,2,\ldots,\frac{M}{K}$ in Step~2.

It is important to note that, the simplification in (\ref{eqn:appb2}) relieves Algorithm~2
from the burden to calculate $NK$ instances of both $s_{nk}$ and $\lambda_l$, and significantly reduces the computational complexity, as shown in Section \ref{sec:compcomp}.

\begin{comment}
It is important to note that, this result relieves Algorithm~2
from the burden to calculate $NK$ instances of both $s_{nk}$ and $\lambda_l$.
\end{comment}
