# Supplementary material for: Discrete Beamforming Optimization for RISs with a Limited Phase Range and Amplitude Attenuation
Source: arXiv:2507.07342 source file (2025-07-09)
Supplement: Supplementary file 2 [file appendixa.tex]

\section{Verification of $N-N'$ Steps When $|{\cal N}(\lambda_l)| \neq 1$}
Assume there are replicas among $s_{nk}$. We know from (\ref{eqn:eqn44}) that there is a positive integer $N'$ such that
\begin{equation}
M = (N-N')K
\label{eqn:eqn48}
\end{equation}
where
\begin{eqnarray}
N' & = & \sum_{m=1}^{{M}/{K}}\left(|{\cal R}_m|-1\right)\\
 & = & \sum_{m=1}^{{M}/{K}} G_m - \frac{M}{K}
\end{eqnarray}
where $G_m = |{\cal R}_m|.$

Replacing $N'$ into (\ref{eqn:eqn48}), we get
\begin{equation}
\sum_{m=1}^{M/K}G_m = N.
\end{equation}
Since there are replicas among $s_{nk},$ there are $m$ for which $G_m>1$, from which $M/K<N$ follows as a necessary condition.

Hence, if $|{\cal N}(\lambda_l)| \neq 1,$ then the global optimum can be reached in $N-N'$ number of steps.
